# Supplementary material for: A Wave Packet Approach to Interacting Fermions
Source: arXiv:1603.04041 source file (2016-03-13)
Supplement: Supplementary file 1 [file wwtrafo2d.tex]

\chapter{Transformation of interactions to WW basis in two dimensions}
\section{Saddle points}
\label{sec:sp_transformation_4M}

\noindent
We derive the approximate transformation from momentum space to the truncated WW basis including states at the saddle points only. The derivation is in one dimension for sake of simplicity, but the generalization to higher dimensions is trivial. The momentum space interactions are known on a discrete grid only, which we take to be oversampled by a factor of two, i.e. $N = 4M$, where $N = \frac{2\pi}{\Delta p}$ is related to the Brillouin zone discretization $\Delta p$. Momentum conservation ensures that the WW momentum $k$ is conserved for the truncated expansion. Hence it is sufficient to treat the couplings $g_1,\ldots,g_4$ separately, and the calculation can be based on the window function
\begin{equation}
g_{2m}(j) \equiv g_{2m, 0}(j)
\end{equation}
and its Fourier transform $\tilde{g}_{2m}(p)$. Since $N=4M$, the possible values of $m$ are $m=0,1$. Relatedly, the allowed values for $p$ are $p = -1, 0, 1$, where we have scaled out a factor of $\frac{2\pi}{N}$ for later convenience. The unshifted window function in momentum space is given by
\begin{equation}
\tilde{g}(p) = \left\{\begin{array}{cc} \frac{1}{\sqrt{2}} & p = 0 \\ \frac{1}{2} & \left| p\right| = 1 \end{array}\right. .
\end{equation}
Applying a shift $2m$ in real space leads to
\begin{eqnarray}
\tilde{g}_{2m}(p) &=& \frac{1}{\sqrt{N}} \sum_j \, e^{-\frac{2\pi}{N} p j} \, g\left(j - 2 M m\right) \nonumber \\
&=& \frac{1}{\sqrt{N}}\sum_j e^{-i\frac{4\pi M}{N} p m} e^{-i\frac{2\pi}{N} p j} g\left(j\right) \nonumber \\
&=& \left(-1\right)^{ p m} \tilde{g}(p),
\end{eqnarray}
where the last line follows from $N=4M$. The transformed interaction is then given by
\begin{equation}
U_{2m_1,\ldots,2 m_4} = \frac{1}{2M}\;\frac{1}{2}\sum_{p_1\cdots p_4} \left(-1\right)^{\sum_{i=1}^4 m_i p_i} \, \left[\prod_{i=1}^4 \tilde{g}\left(p_i\right)\right] \,\delta_{p_1+p_2,p_3+p_4} U\left(p_1,p_2,p_3\right),
\end{equation}
where $U\left(p_1,p_2,p_3\right)$ is the renormalized momentum space interaction. The generalization to the two-dimensional saddle point system is 
\begin{eqnarray}
U^{a_1\cdots a_4}_{2\mathbf{m}_1,\ldots,2\mathbf{m}_4} &=& \frac{1}{\left(2M\right)^2}\;\frac{1}{4} \sum_{\mathbf{p}_1\cdots \mathbf{p}_4} \left(-1\right)^{\sum_{i=1}^4 \mathbf{m}_i\cdot \mathbf{p}_i} \left[\prod_{i=1}^4\tilde{G}\left(\mathbf{p}_{i}\right)\right]\, \delta_{\mathbf{p}_1 + \mathbf{p}_2,\mathbf{p}_3+\mathbf{p}_4} \nonumber \\&&\;\times \;U\left(\mathbf{p}^{(a_1)}+\mathbf{p}_1,\mathbf{p}^{(a_2)}+\mathbf{p}_2,\mathbf{p}^{(a_3)}+\mathbf{p}_3\right).
\label{eq:sp_transformation_4M}
\end{eqnarray}
Note that for $\mathbf{p}_i=0$ all momenta lie at one of the saddle points. In order to use the interaction for a larger lattice, the periodic boundary conditions have to be taken into account, and all non-local interactions have to be divided by the number of bonds connecting the sites. Hence nearest neighbor interactions have to be multiplied by $\frac{1}{2}$, and next-to-nearest neighbor interactions by $\frac{1}{4}$.

\section{Other states on the umklapp surface}
\label{sec:gen_transformation_4M}

\noindent
The formula for the transformation of interactions for states other than the saddle point states is different because $k_i \neq 0,M$, so that the WW basis states are given by
\begin{equation}
\Psi_{\mathbf{m},\mathbf{k}}\left(\mathbf{j}\right) = \frac{1}{2} \sum_{\al} e^{-i\al\cdot\Phi_{\mathbf{m}+\mathbf{k}}} G_{\mathbf{m}, A_{\al}\mathbf{k}}\left(\mathbf{j}\right),
\end{equation}
where 
\begin{equation}
A_{\al} = \left(\begin{array}{cc} \alpha_1 & 0 \\ 0 & \alpha_2 \end{array}\right).
\end{equation}

\noindent

\begin{eqnarray}
U_{\mathbf{m}_1\cdots \mathbf{m}_4} &=& \frac{1}{16} \sum_{\al_1\cdots \al_4} e^{-i\left(\al_1\cdot \Phi_{\mathbf{m}_1} + \al_2\cdot \Phi_{\mathbf{m_2}} -\al_3\cdot \Phi_{\mathbf{m}_3} - \al_4\cdot \Phi_{\mathbf{m_4}}\right)} \delta_{\al_1+\al_2,\al_3+\al_4} \, \nonumber \\&& \times \, \frac{1}{N^2}\sum_{\mathbf{p}_1\cdots \mathbf{p}_4} \, e^{-i M\left(\mathbf{m}_1\cdot \mathbf{p}_1 + \mathbf{m}_2\cdot \mathbf{p}_2 - \mathbf{m}_3\cdot \mathbf{p}_3 - \mathbf{m}_4\cdot \mathbf{p}_4\right)} \delta_{\mathbf{p}_1+\mathbf{p}_2,\mathbf{p}_3+\mathbf{p}_4} \nonumber \\ && \times \;U\left(\mathbf{p}^{(\al_1)}+\mathbf{p}_1,\mathbf{p}^{(\al_2)}+\mathbf{p}_2,\mathbf{p}^{(\al_3)}+\mathbf{p}_3\right) \; \prod_{i=1}^4 \tilde{G}\left(\mathbf{p}_i\right).
\end{eqnarray}
