# Supplementary material for: A Wave Packet Approach to Interacting Fermions
Source: arXiv:1603.04041 source file (2016-03-13)
Supplement: Supplementary file 2 [file operator_trafo.tex]

\chapter{Details for the transformation of operators in one dimension}
\label{app:operator_trafo}

\section{Kinetic energy}
\noindent
In this section we discuss the WW representation of the kinetic energy operator
\begin{equation}
\ham{kin} = \sum_p \epsilon(p) c^\dagger_p\, c^\pdag_p,
\end{equation}
where we assume $\epsilon_p = -2t\cos p$ in the following (more general forms of the dispersion can be dealt with in the same manner, however). $t$ is the hopping rate for nearest neighbor hopping, the bandwidth is $W=4t$.  
\noindent
The wave packet transform of $\epsilon(p)$ by $\bar{T}(m\alpha k,m'\alpha'k')$. We define
\begin{equation}
q_\pm = \frac{\pi}{2M} \left(\alpha k - \alpha'k'\right),
\end{equation}
where $q_{+}$ is the average of the momenta of the two wave packets and $2q_{-}$ is their difference.
From (\ref{eq:O_wave_packet_transform}) we obtain
\begin{eqnarray}
\bar{T}\left(m\alpha k,m'\alpha'k'\right) &=& -2t \sum_{p} \epsilon\left(p+q_{+} \right) \, e^{-iM p\left(m - m' \right)} \, e^{-iM q_{-} \left(m+m'\right)} \,\tilde{g}\left(p+q_{-}\right)\tilde{g}\left(p-q_{-}\right)
\label{eq:T_wave_packet}
\end{eqnarray}
From the momentum space localization of $\tilde{g}(p)$ it follows that for $\left|\alpha k-\alpha'k'\right| > 1$, the RHS of (\ref{eq:T_wave_packet}) vanishes.

\section{Interaction}
